# Supplementary material for: Towards more patient friendly clinical notes through language models and ontologies
Source: arXiv:2112.12672 source file (2021-12-23)
Supplement: Supplementary file 1 [file appendix.tex]

\newpage
\onecolumn
\appendix
\setcounter{table}{0}

\section{Appendices}
\label{sec:appendix}
%Appendices are material that can be read, and include lemmas, formulas, proofs, and tables that are not critical to the reading and understanding of the paper. 
%Appendices should be \textbf{uploaded as supplementary material} when submitting the paper for review. Upon acceptance, the appendices come after the references, as shown here. Use
% \verb|\appendix|

\subsection{Example sentences}

Table \ref{tab:exampleSents} shows an extract of the dataset, together with the simplified sentences from our best model.
\begingroup

\begin{table*}[tbhp]
    \centering
    \caption{Examples sentences (original, our best model, human reference)}
    \small
        \begin{tabular}{ |p{4.5cm}|p{4.5cm}|p{4.5cm}|  }
        \hline
        \multicolumn{1}{|c|}{\textbf{Original/Reference sentence}} & \multicolumn{1}{|c|}{\textbf{GPT-1 simplified sentence}} & \multicolumn{1}{|c|}{\textbf{Clinician simplified sentence}}  \\
        \hline
        No hemorrhage is identified. & No blood loss is identified. & No bleeding is identified. \\
        Myocardial infarction can not be excluded. & Heart attack can not be excluded. & Heart attack can not be excluded . \\
        Two days later, the pain resolved and she has not had a recurrence. & Two days later, the pain resolved and she has not had a recurrence. & Two days later, the pain got better and she has not had a recurrence. \\
        He then had a tracheostomy placed.    & He then had a tracheostomy placed. & He then had a breathing tube placed. \\
        Skin : No rashes. & Skin : No spots on skin. & Skin : No rashes. \\
        There was minimal associated edema and no mass effect. & There was minimal associated fluid retention and no mass effect. & There 
        was minimal associated swelling and no mass effect.   \\
        \hline
        \end{tabular}
    \label{tab:exampleSents}
\end{table*}
\endgroup

% \subsection{Human Evaluation with Majority Vote Answers}
% \input{tables/appendix_contingency.tex}
% \input{tables/appendix_significance.tex}

\subsection{Medical simplification instructions}
\label{sec:simplification-guidelines}
\paragraph{Overview:}
The purpose of this task is to simplify sentences that contain medical content so that patients are able to understand them.
\paragraph{Step 1:}
    In the first column decide whether you think this sentence needs to be made simpler.
Reasons for \emph{not} making a sentence simpler are:
\begin{itemize}
    \item The sentence contains no real content or insufficient context e.g. a stand-alone blood test result or numeric value.
    \item The sentence is too specific e.g. a post operative note with detail on procedure/hardware used.
    \item The majority of the sentence is made up of drug names and/or brand names.
\end{itemize}
\paragraph{Step 2:}
     If the sentence is deemed suitable for simplification, please write a simpler version of the sentence that a lay person would understand. Guidelines for simplification are:

% \paragraph{Guidelines for simplification}
\begin{itemize}
    \item Re-write the sentence using easy-to-understand terms while maintaining the medical context and content.
    \item Keep the sentence as close to the original structure as possible.
    \item Retain the tense of the sentence.
\end{itemize}

\subsection{Mechanical Turk guidelines}
\paragraph{Task description:}

The sentences are taken from medical discharge letters. You don't need to worry too much about small grammatical errors (i.e., punctuation in the wrong place, etc.); instead you should focus on the meaning and how well you understand it. Imagine reading the sentence in a letter from your doctor: Would you understand what s/he means?

\paragraph{}
You will be presented with sentence A and sentence B. You should first read the sentences carefully and ensure that you attempt to understand the meaning behind it.

\paragraph{Question:}
Which sentence is easier to understand? Please, choose one of the categories depending how well you understand sentence B compared to sentence A (even if the difference is only small).
\begin{enumerate}
    \item Sentence A is easier to understand.

    \item Sentence B is easier to understand.

    \item I understand them both the same amount.

    \item I do not understand either of these sentences.
\end{enumerate}

\paragraph{Rules \& tips:}
 Take time to read the sentences and attempt to understand the meaning behind them.
\subsection{Grammaticality preservation guidelines}
\begin{itemize}
\paragraph{Scoring criteria:}
    \item No errors - No additional errors have been introduced or only punctuation/capitalisation errors
    \item Minor errors introduced - Would require minor changes to correct i.e. the addition, deletion or substitution of prepositions or particles, or minor morphological changes
    \item Major errors introduced - Would require substantial changes to correct i.e. significant re-organisation of the sentence, many morphological changes or the introduction/removal of content words 
\end{itemize}
\subsection{Convergence Ablation Study}
\begin{table*}[h]
    \centering
    \caption{Convergence Ablation. Human judgement counts for sentence pairs from the test set for all models sentences. \textbf{S:} the generated was simpler; \textbf{F:} the original was simpler; \textbf{E:} both of equal complexity; \textbf{N:} cannot understand either; \textbf{SG:} simplification gain as defined in Equation \ref{eq:ratio}. Bold indicates best model.}

    \begin{tabular}{k|jjjj|j}
              \multicolumn{1}{s}{~} &
              \multicolumn{1}{s}{\textbf{S}}    & \multicolumn{1}{s}{\textbf{F}}    & \multicolumn{1}{s}{\textbf{E}}    & \multicolumn{1}{s}{\textbf{N}}    & \multicolumn{1}{s}{\textbf{SG}}    \\
        \hline
        \hline
        n-gram  (converged) & \textcolor{OliveGreen}{200} & \textcolor{BrickRed}{\textbf{146}} & 196 & \textbf{11}  & \textcolor{NavyBlue}{\textbf{0.031}}  \\
        n-gram (1st iteration) & \textcolor{OliveGreen}{\textbf{203}} & \textcolor{BrickRed}{159} & \textbf{174} & 17 & \textcolor{NavyBlue}{0.025}  \\
        \hline
        
        GPT-1  (converged) & \textcolor{OliveGreen}{263} & \textcolor{BrickRed}{\textbf{193}}  & 349 & \textbf{21}  & \textcolor{NavyBlue}{\textbf{0.040}} \\
        GPT-1  (1st iteration) & \textcolor{OliveGreen}{\textbf{285}} & \textcolor{BrickRed}{218}  & \textbf{294} & 29 & \textcolor{NavyBlue}{0.038} \\
        \hline

        GPT-2  (converged) & \textcolor{OliveGreen}{235} & \textcolor{BrickRed}{218} & \textbf{247} & \textbf{14} & \textcolor{NavyBlue}{0.010}\\
        GPT-2  (1st iteration) & \textcolor{OliveGreen}{\textbf{237}} & \textcolor{BrickRed}{\textbf{208}} & 285 & 19 & \textcolor{NavyBlue}{\textbf{0.016}}\\
    \end{tabular}
    \label{tab:convergence_ablation}
\end{table*}

            % \todo{Compute Simplification Gain, somehow...}

\subsection{Significance Tests}
\label{sec:significance-tests}
\begin{table}[h]
    \centering
        \caption{Results of approximate randomisation significance tests \cite{Efron1987} on simplification gain $SG$ scores presented in Table \ref{tab:human_eval}}
\begin{tabular}{k|jjjj}
              \multicolumn{1}{s}{~} &
              \multicolumn{1}{s}{\textbf{n-gram}}    & \multicolumn{1}{s}{\textbf{GPT-1}}    & \multicolumn{1}{s}{\textbf{GPT-2}}    & \multicolumn{1}{s}{\textbf{NTS}}    \\
        \hline
        \hline
        Human   & 0.000** & 0.000** & 0.000** & 0.000** \\ 
        \hline
        n-gram  & \multicolumn{1}{s}{\textbf{-}} & 0.000** & 0.025* & 0.000** \\
        GPT-1   & \multicolumn{1}{s}{\textbf{-}} & \multicolumn{1}{s}{\textbf{-}} & 0.000** & 0.000** \\
        GPT-2   & \multicolumn{1}{s}{\textbf{-}} & \multicolumn{1}{s}{\textbf{-}} & \multicolumn{1}{s}{\textbf{-}} & 0.000** \\
        \hline
        \multicolumn{2}{s}{\textsuperscript{**} $p<0.01$, 
      \textsuperscript{*} $p<0.05$}
    \end{tabular}
    \label{tab:significance_SG}
\end{table}
