# Supplementary material for: Towards more patient friendly clinical notes through language models and ontologies
Source: arXiv:2112.12672 source file (2021-12-23)
Supplement: Supplementary file 2 [file appendix_contingency.tex]

\begin{table*}[htbp]
    \centering
    \small
        \begin{tabular}{lc|cccccccc}
            \hline
            \multicolumn{1}{l}{\textbf{Measure}}  &  
            \multicolumn{1}{l}{\textbf{Ref.}}  &
            \multicolumn{1}{l}{\textbf{n-gram}}  &
            \multicolumn{1}{l}{\textbf{GPT1}}  &
            \multicolumn{1}{l}{\textbf{GPT2-G}}  &
            \multicolumn{1}{l}{\textbf{NMT}}  \\
            \hline
            1 – Simpler than orig. & \textcolor{OliveGreen}{\textbf{283}} & \textcolor{OliveGreen}{\textbf{168}} & \textcolor{OliveGreen}{162} & \textcolor{OliveGreen}{163} & \textcolor{OliveGreen}{34} \\
            (SimpleScore) & \textcolor{OliveGreen}{\textbf{\emph{\scriptsize{78.18\%}}}} & \textcolor{OliveGreen}{\textbf{\emph{\scriptsize{36.60\%}}}} & \textcolor{OliveGreen}{\emph{\scriptsize{36.9\%}}} & \textcolor{OliveGreen}{\emph{\scriptsize{35.67\%}}} & \textcolor{OliveGreen}{\emph{\scriptsize{13.13\%}}} \\

            2 – harder than orig. & \textcolor{BrickRed}{\textbf{11}} & \textcolor{BrickRed}{79} & \textcolor{BrickRed}{\textbf{37}} & \textcolor{BrickRed}{93} & \textcolor{BrickRed}{96} \\
            & \textcolor{BrickRed}{\textbf{\emph{\scriptsize{3.04\%}}}} & \textcolor{BrickRed}{\emph{\scriptsize{17.21\%}}} & \textcolor{BrickRed}{\textbf{\emph{\scriptsize{8.43\%}}}} & \textcolor{BrickRed}{\emph{\scriptsize{20.35\%}}} & \textcolor{BrickRed}{\emph{\scriptsize{37.07\%}}} \\

            3 – same level & 67 & 211 & 238 & 199 & 129 \\
            & \emph{\scriptsize{18.51\%}} & \emph{\scriptsize{45.97\%}} & \emph{\scriptsize{54.21\%}} & \emph{\scriptsize{43.54\%}} & \emph{\scriptsize{49.81\%}} \\
            
            4 – equally hard & 1 & 1 & 2 & 2 & 0 \\
            & \emph{\scriptsize{0.28\%}} & \emph{\scriptsize{0.22\%}} & \emph{\scriptsize{0.46\%}} & \emph{\scriptsize{0.44\%}} & \emph{\scriptsize{0.00\%}} \\
            \hline
            
            RatioScore & \textcolor{NavyBlue}{\textbf{272}} & \textcolor{NavyBlue}{89} & \textcolor{NavyBlue}{\textbf{125}} & \textcolor{NavyBlue}{70} & \textcolor{NavyBlue}{-62}\\

            \hline
        \end{tabular}
    \caption{Human evaluation of simplification models based on majority voted categories with a minimum majority count of 4}
    \label{tab:appendix_contigency}
\end{table*}
