# Supplementary material for: Towards more patient friendly clinical notes through language models and ontologies
Source: arXiv:2112.12672 source file (2021-12-23)
Supplement: Supplementary file 3 [file appendix_significance.tex]

\begin{table*}[htbp]
    \centering
    \begin{tabular}{l l l l l}
      & \textbf{ngram} & \textbf{GPT1} & \textbf{GPT2-G} & \textbf{NMT}\\ 
    \hline
    Ref & 0.000** & 0.000** & 0.000** & 0.000** \\
    ngram &  & 0.001** & 0.594 & 0.000** \\
    GPT1 &  & & 0.012* & 0.000** \\
    GPT2-G &  &  &  & 0.000** \\
    \hline
    \multicolumn{3}{l}{\textsuperscript{**}$p<0.01$, 
      \textsuperscript{*}$p<0.05$}
\end{tabular}
\caption{P-values obtained from Chi-squared significance test on Majority-vote answer contingency table.}
\label{tab:appendix_significance}
\end{table*}
